# Supplementary material for: Sharpness-Aware Minimization Revisited: Weighted Sharpness as a Regularization Term
Source: arXiv:2305.15817 source file (2024-12-05)
Supplement: Supplementary file 1 [file appendix.tex]

\section*{Appendix}
\section{Code of WSAM}
The code is modified from \url{https://github.com/davda54/sam}.

\lstset{
    language=Python,
    aboveskip=1em,
    breaklines=true,
    abovecaptionskip=-6pt,
    captionpos=b,
    escapeinside={\%*}{*)},
    frame=single,
    numbers=left,
    numbersep=15pt,
    numberstyle=\tiny,
}

\begin{lstlisting}[frame=single]
import torch
import contextlib
import torch.distributed as dist
# Please refer to `davda54/sam' for the utils code below
from utility.bypass_bn import enable_running_stats, disable_running_stats


class WeightedSAM(torch.optim.Optimizer):
    def __init__(
        self,
        model,
        base_optimizer,
        rho=0.05,
        gamma=0.5,
        sam_eps=1e-12,
        adaptive=False,
        decouple=True,
        **kwargs,
    ):
        assert rho >= 0.0, f"Invalid rho, should be non-negative: {rho}"

        self.model = model
        self.base_optimizer = base_optimizer
        self.decouple = decouple
        alpha = gamma / (1 - gamma)
        defaults = dict(
            rho=rho, alpha=alpha, sam_eps=sam_eps, adaptive=adaptive, **kwargs
        )
        defaults.update(self.base_optimizer.defaults)
        super(WeightedSAM, self).__init__(self.base_optimizer.param_groups, defaults)

    @torch.no_grad()
    def first_step(self, zero_grad=False):
        grad_norm = self._grad_norm()
        for group in self.param_groups:
            scale = group["rho"] / (grad_norm + group["sam_eps"])

            for p in group["params"]:
                if p.grad is None:
                    continue
                e_w = (
                    (torch.pow(p, 2) if group["adaptive"] else 1.0)
                    * p.grad
                    * scale.to(p)
                )
                p.add_(e_w)  # climb to the local maximum "w + e(w)"
                self.state[p]["old_p"] = p.data.clone()
                self.state[p]["grad"] = p.grad.detach().clone()
        if zero_grad:
            self.zero_grad()

    @torch.no_grad()
    def second_step(self, zero_grad=False, clip_grad_norm=None):
        for group in self.param_groups:
            for p in group["params"]:
                if p.grad is None:
                    continue
                p.data = self.state[p]["old_p"]
                if torch.distributed.is_initialized():
                    dist.all_reduce(self.state[p]["grad"], op=dist.ReduceOp.AVG)
                if not self.decouple:
                    p.grad.mul_(group["alpha"]).add_(
                        self.state[p]["grad"], alpha=1.0 - group["alpha"]
                    )
                else:
                    self.state[p]["sharpness"] = (
                        p.grad.detach().clone() - self.state[p]["grad"]
                    )
                    p.grad.mul_(0.0).add_(self.state[p]["grad"], alpha=1.0)

        if clip_grad_norm is not None:
            torch.nn.utils.clip_grad_norm_(self.model.parameters(), clip_grad_norm)
        self.base_optimizer.step()  # do the actual "sharpness-aware" update

        if self.decouple:
            for group in self.param_groups:
                for p in group["params"]:
                    if p.grad is None:
                        continue
                    p.add_(
                        self.state[p]["sharpness"], alpha=-group["lr"] * group["alpha"]
                    )

        if zero_grad:
            self.zero_grad()

    def maybe_no_sync(self):
        if torch.distributed.is_initialized():
            return self.model.no_sync()
        else:
            return contextlib.ExitStack()

    @torch.no_grad()
    def step(self, closure=None):
        assert (
            closure is not None
        ), "Sharpness Aware Minimization requires closure, but it was not provided"
        closure = torch.enable_grad()(
            closure
        )  # the closure should do a full forward-backward pass

		with self.maybe_no_sync():
			enable_running_stats(self.model)
			loss = closure()
        self.first_step(zero_grad=True)

        disable_running_stats(self.model)
        closure()
        self.second_step()

        return loss

    def _grad_norm(self):
        shared_device = self.param_groups[0]["params"][
            0
        ].device  # put everything on the same device, in case of model parallelism
        norm = torch.norm(
            torch.stack(
                [
                    ((torch.abs(p) if group["adaptive"] else 1.0) * p.grad)
                    .norm(p=2)
                    .to(shared_device)
                    for group in self.param_groups
                    for p in group["params"]
                    if p.grad is not None
                ]
            ),
            p=2,
        )
        return norm
\end{lstlisting}
